# Supplementary material for: Geometry and physics in the deformations of crystalline caps
Source: arXiv:2207.10233 source file (2022-07-21)
Supplement: Supplementary file 1 [file SI-compressed.pdf]

# Supplemental Material

Jingyuan Chen and Zhenwei Yao\*

*School of Physics and Astronomy, and Institute of Natural Sciences,*

*Shanghai Jiao Tong University, Shanghai 200240, China*

## I. SIMULATION DETAILS

We implement the fixed boundary condition by anchoring the particles within the boundary annulus of width  $3r_m$ .  $r_m$  is the equilibrium distance of the Lennard-Jones potential. The array of the L-J particles confined on the sphere of radius  $R$  is relaxed by the steepest descent method [1, 2]. To fully and efficiently relax the system, we first update the particle configuration collectively, and then update the positions of individual particles by the fine step at the order of  $10^{-5}r_m$ . In the numerically obtained lowest-energy configurations, the magnitude of the residual force on each particle is typically at the order of  $10^{-5}\epsilon_0/r_m$ . With the shrinking of the sphere, the particle configuration in mechanical equilibrium is projected to the smaller sphere along the z-axis, which is defined to be the line connecting the centers of the sphere and the cap. The particles within the boundary annulus are still anchored on the smaller sphere. The typical shrinking rate of the sphere is  $\delta R = 0.2r_m$ , under which the variation of the lattice spacing caused by the projection is within  $4 \times 10^{-3}r_m$  in our simulations. Near the yield transition, the sphere is controlled to shrink in a finer step of  $\delta R = 0.01r_m$ .

The value for the Poisson's ratio of a pre-stressed triangular lattice is obtained by numerical simulations according to the definition of Poisson's ratio. Specifically, by imposing a pair of forces along the  $x$ -axis on the opposite edges of a square-shaped triangular L-J lattice, a strain field of  $(u_{xx}^{(0)}, u_{yy}^{(0)})$  is created over the lattice in mechanical equilibrium.  $u_{xx}^{(0)} \neq 0$  and  $u_{yy}^{(0)} = 0$ . The mechanical relaxation of the lattice is realized by the standard steepest descent method. [1, 2] By the definition of Poisson's ratio,  $\nu = -\delta u_{yy}/\delta u_{xx}$ , where  $-\delta u_{yy}$  indicates the amount of relative transverse shrinking in response to small longitudinal ex-

---

\*Electronic address: zyao@sjtu.edu.cn

tension ( $\delta u_{xx}$ ) by slightly pulling the pre-stressed lattice along the  $x$ -axis. [3, 4] Both  $\delta u_{yy}$  and  $\delta u_{xx}$  are on the order of  $10^{-4}$  in simulations.

## II. THEORETICAL ANALYSIS

In this section, we present the derivations of relevant equations in the main text. The elastic deformation of the crystalline cap on the sphere is treated analytically by the continuum elasticity theory. The crystalline cap is modeled as a two-dimensional isotropic continuum elastic medium with Young's modulus  $Y$  and Poisson's ratio  $\nu$  [3]. The constitutive relations are

$$\sigma_{\rho\rho} = \frac{Y}{1-\nu^2}(u_{\rho\rho} + \nu u_{\varphi\varphi}), \quad (1)$$

$$\sigma_{\varphi\varphi} = \frac{Y}{1-\nu^2}(u_{\varphi\varphi} + \nu u_{\rho\rho}). \quad (2)$$

where  $\sigma_{\alpha\beta}$  and  $u_{\alpha\beta}$  are the stress and strain tensors.

### A. Approximate solution to the FvK equations

Under the small deformation approximation, the stress distribution over the crystalline cap in mechanical equilibrium is governed by the Föppl-von Kármán(FvK) equations [3]. The FvK equations consist of a pair of force balance equations in the tangent and normal directions. We solve for the in-plane stress field by analyzing the FvK equation in the tangential direction.

In the polar coordinates  $(\rho, \varphi)$ , the  $\hat{e}_\rho$ - and  $\hat{e}_\varphi$ -components of the FvK equation read as [3]:

$$\partial_\rho \sigma_{\rho\rho} + \frac{1}{\rho}(\partial_\varphi \sigma_{\rho\varphi} + \sigma_{\rho\rho} - \sigma_{\varphi\varphi}) = 0, \quad (3)$$

$$\partial_\rho \sigma_{\rho\varphi} + \frac{1}{\rho}(\partial_\varphi \sigma_{\varphi\varphi} + 2\sigma_{\rho\varphi}) = 0. \quad (4)$$

By making use of the rotational symmetry of the system, Eqs.(3) and (4) are reduced to

$$\partial_\rho \sigma_{\rho\rho} + \frac{1}{\rho}(\sigma_{\rho\rho} - \sigma_{\varphi\varphi}) = 0, \quad (5)$$

$$\sigma_{\rho\varphi} = 0. \quad (6)$$

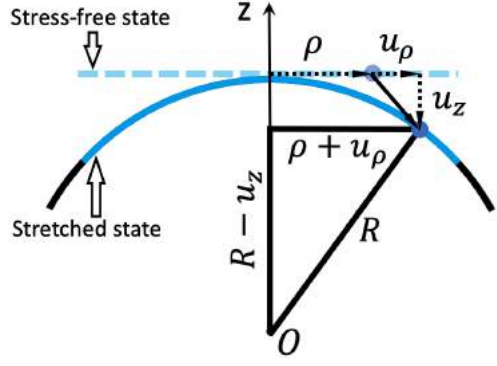

FIG. 1: Schematic plot of the deformation from the planar disk (dashed blue line) to the spherical crystalline cap (solid blue curve).  $u_\rho$  and  $u_z$  are the components of the displacement vector.

The particles within the boundary annulus are anchored, which is formulated as the fixed boundary condition:  $u_\rho(\rho = \rho_0) = 0$ . Due to the rotational symmetry, we have  $u_\rho(\rho = 0) = 0$ . To conveniently deal with these boundary conditions, we express the force balance equations in terms of the displacement vector, whose components  $u_\rho$  and  $u_z$  are shown in Fig. 1. To this end, we first establish the relation between the strain tensor and the displacement vector under the small displacement approximation [5]:

$$u_{\rho\rho} = \partial_\rho u_\rho + \frac{1}{2}(\partial_\rho u_z)^2, \quad (7)$$

$$u_{\varphi\varphi} = \frac{u_\rho}{\rho}, \quad (8)$$

By further inserting Eqs. (1),(2),(7), (8) to Eq. (5), we obtain the force balance equation in terms of the displacement vector:

$$\frac{d^2 u_\rho}{d\rho^2} + \frac{1}{\rho} \left( \frac{du_\rho}{d\rho} - \frac{u_\rho}{\rho} \right) + \frac{1}{2} \frac{d}{d\rho} \left[ \left( \frac{du_z}{d\rho} \right)^2 \right] + \frac{1-\nu}{2\rho} \left( \frac{du_z}{d\rho} \right)^2 = 0. \quad (9)$$

Now, we analytically solve Eq. (9). First, from the following geometric constraint condition as shown in Fig. 1:

$$[\rho + u_\rho(\rho)]^2 + [R - u_z(\rho)]^2 = R^2, \quad (10)$$

we have  $du_z/d\rho = \rho/R$  under the small deformation approximation. By applying the boundary condition of  $u_\rho(\rho = 0) = u_\rho(\rho = \rho_0) = 0$ , we obtain the solution to Eq.(9):

$$u_\rho(\rho) = \frac{3-\nu}{16} \frac{\rho_0^3}{R^2} \left[ \frac{\rho}{\rho_0} - \left( \frac{\rho}{\rho_0} \right)^3 \right]. \quad (11)$$

By inserting Eq. (11) into Eqs.(7) and (8), we finally have

$$u_{\rho\rho} = \frac{3-\nu}{16} \frac{\rho_0^2}{R^2} + \frac{3\nu-1}{16} \frac{\rho_0^2}{R^2} \left( \frac{\rho}{\rho_0} \right)^2, \quad (12)$$

$$u_{\varphi\varphi} = \frac{3-\nu}{16} \frac{\rho_0^2}{R^2} + \frac{\nu-3}{16} \frac{\rho_0^2}{R^2} \left( \frac{\rho}{\rho_0} \right)^2. \quad (13)$$

## B. Higher-order approximation

To obtain higher order terms in the analytical expressions for the strain field in Eqs.(12) and (13), we express the in-plane force balance equation on the deformed spherical cap in spherical coordinates  $(\theta, \phi)$ . The  $\hat{e}_\theta$ - and  $\hat{e}_\phi$ -components of the in-plane force balance equation read as

$$\partial_\theta \sigma_{\theta\theta} + \partial_\phi \left( \frac{\sigma_{\theta\phi}}{\sin \theta} \right) + \cot \theta (\sigma_{\theta\theta} - \sigma_{\phi\phi}) = 0, \quad (14)$$

$$\partial_\theta \sigma_{\theta\phi} + \frac{1}{\sin \theta} \partial_\phi \sigma_{\phi\phi} + 2 \cot \theta \sigma_{\theta\phi} = 0. \quad (15)$$

Due to the rotational symmetry of the system, Eqs.(14) and (15) are reduced to

$$\frac{d\sigma_{\theta\theta}}{d\theta} + \cot \theta (\sigma_{\theta\theta} - \sigma_{\phi\phi}) = 0, \quad (16)$$

$$\sigma_{\theta\phi} = 0. \quad (17)$$

Similar to the procedure in the previous subsection, in the following we shall express the force balance equation in terms of the displacement vector. We first establish the exact relation between the strain tensor and the displacement vector [5], which contains higher order nonlinear terms in comparison with Eq.(7):

$$u_{\rho\rho} = \partial_\rho u_\rho + \frac{1}{2} [(\partial_\rho u_\rho)^2 + (\partial_\rho u_z)^2], \quad (18)$$

$$u_{\varphi\varphi} = \frac{u_\rho}{\rho} + \frac{u_\rho^2}{2\rho^2}, \quad (19)$$

We further express Eqs.(16) and (17) in polar coordinates  $(\rho, \varphi)$ , which are established in the undeformed planar disk. The transformation of the spherical and polar coordinates is characterized by the displacement  $u_\rho$ :

$$\sin \theta = \frac{\rho + u_\rho}{R}, \quad (20)$$

$$\phi = \varphi, \quad (21)$$

By making use of Eqs.(20) and (21), Eqs.(16) and (17) are rewritten as

$$\frac{d\sigma_{\rho\rho}}{d\rho} + \frac{1}{\rho + u_\rho} \left(1 + \frac{du_\rho}{d\rho}\right) (\sigma_{\rho\rho} - \sigma_{\varphi\varphi}) = 0, \quad (22)$$

$$\sigma_{\rho\varphi} = 0. \quad (23)$$

By inserting Eqs. (18),(19) and the constitutive relations [Eqs. (1),(2)] into Eq. (22), we have

$$\begin{aligned} & \left(1 + \frac{du_\rho}{d\rho}\right) \frac{d^2 u_\rho}{d\rho^2} + \frac{\nu}{\rho} \left(1 + \frac{u_\rho}{\rho}\right) \left(\frac{du_\rho}{d\rho} - \frac{u_\rho}{\rho}\right) + \frac{1}{2} \frac{d}{d\rho} \left[\left(\frac{du_z}{d\rho}\right)^2\right] \\ & + \frac{(1-\nu)}{2(\rho + u_\rho)} \left(1 + \frac{du_\rho}{d\rho}\right) \left[\left(2 + \frac{du_\rho}{d\rho}\right) \frac{du_\rho}{d\rho} - \left(2 + \frac{u_\rho}{\rho}\right) \frac{u_\rho}{\rho} + \left(\frac{du_z}{d\rho}\right)^2\right] = 0. \end{aligned} \quad (24)$$

By applying the boundary condition of  $u_\rho(\rho = 0) = u_\rho(\rho = \rho_0) = 0$  and the geometric constraint Eq. (10), we obtain the solution to Eq.(24) up to  $(\rho_0/R)^4$ :

$$u_\rho(\rho) = \frac{3-\nu}{16} \frac{\rho_0^3}{R^2} \left[\frac{\rho}{\rho_0} - \left(\frac{\rho}{\rho_0}\right)^3\right] + 3 \left(\frac{3-\nu}{16}\right)^2 \frac{\rho_0^5}{R^4} \left[\frac{\rho}{\rho_0} - \left(\frac{\rho}{\rho_0}\right)^3\right], \quad (25)$$

which contains higher order terms in comparison with Eq. (11). By inserting Eq. (25) into Eqs. (18) and (19), we finally obtain the analytical expression for the strain field up to  $(\rho_0/R)^4$ :

$$u_{\rho\rho} = \frac{3-\nu}{16} \frac{\rho_0^2}{R^2} + \frac{7(3-\nu)^2}{512} \frac{\rho_0^4}{R^4} + \left[\frac{3\nu-1}{16} \frac{\rho_0^2}{R^2} - \frac{(1-3\nu)(3-\nu)}{64} \frac{\rho_0^4}{R^4}\right] \left(\frac{\rho}{\rho_0}\right)^2, \quad (26)$$

$$u_{\varphi\varphi} = \frac{3-\nu}{16} \frac{\rho_0^2}{R^2} + \frac{7(3-\nu)^2}{512} \frac{\rho_0^4}{R^4} + \left[\frac{\nu-3}{16} \frac{\rho_0^2}{R^2} - \frac{(3-\nu)^2}{64} \frac{\rho_0^4}{R^4}\right] \left(\frac{\rho}{\rho_0}\right)^2. \quad (27)$$

In comparison with the conventional approximate solutions to the FvK equations [see Eqs. (12) and (13)], the higher order terms in Eqs. (26) and (27) significantly reduce the gap between the analytical results based on the FvK equations and the simulation data as shown in Fig.1(c) in the main text. Equations (26) and (27) show that the homogeneous substrate geometry could create an inhomogeneous strain field, which is fundamentally different from the case of a planar membrane under radial tension.

### III. QUASI-CONFORMAL ORDERING AND THE INDUCED GAUSSIAN CURVATURE

In this section, we provide more information about the analysis of the inhomogeneous deformed lattice, including the distribution of the bond angle and the derivation for the

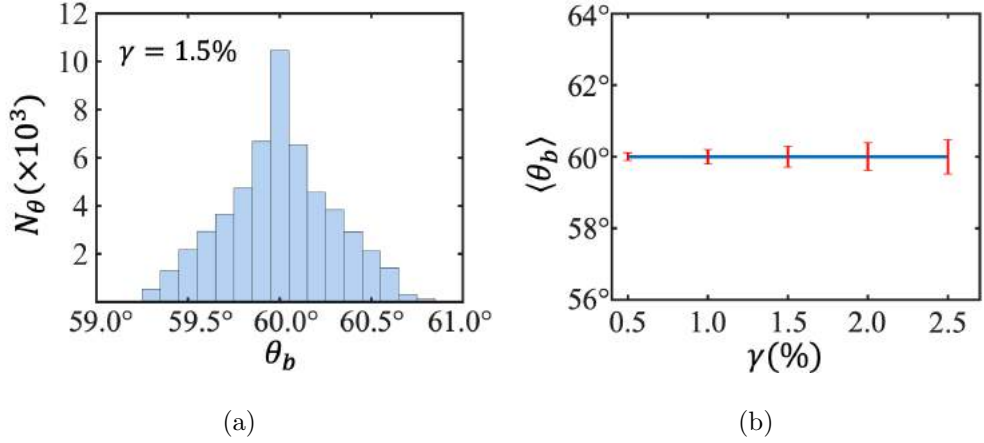

FIG. 2: The bond angle distribution in the deformed lattice on the sphere. (a) A typical histogram plot at  $\gamma = 1.5\%$ .  $R = 170.1r_m$ . (b) The dependence of the mean bond angle on the degree of stretching  $\gamma$ .  $\rho_0 = 50r_m$ .

relation between the induced Gaussian curvature  $K_\ell$  and the strain tensor under the small deformation approximation. We also discuss the density distribution under which the substrate curvature is fully screened by  $K_\ell$ .

### A. Bond angle distribution

The distribution of the bond angle for a typical stretched crystalline cap at  $\gamma = 1.5\%$  is presented in Fig. 2(a). We observe that the distribution of the bond angle is sharply concentrated at  $60^\circ$ . The dependence of the mean bond angle on the degree of stretching is plotted in Fig. 2(b). It clearly shows that the deformation is approximately angle-preserved. Consequently, the deformed triangular lattice consists of quasi-equilateral triangles. The revealed quasi-conformal ordering constitutes the foundation for the further analysis of the underlying curvature structure in the deformed lattice. Note that it is impossible to construct a strictly conformal crystal over the sphere according to the connection of the total interior angle of spherical triangles and the integrated curvature [6].

### B. The relation between the induced curvature and the strain tensor

The quasi-conformal ordering in the deformed lattice allows us to construct the metric on the undeformed planar disk as in Eq.(5) in the main text, from which one could derive

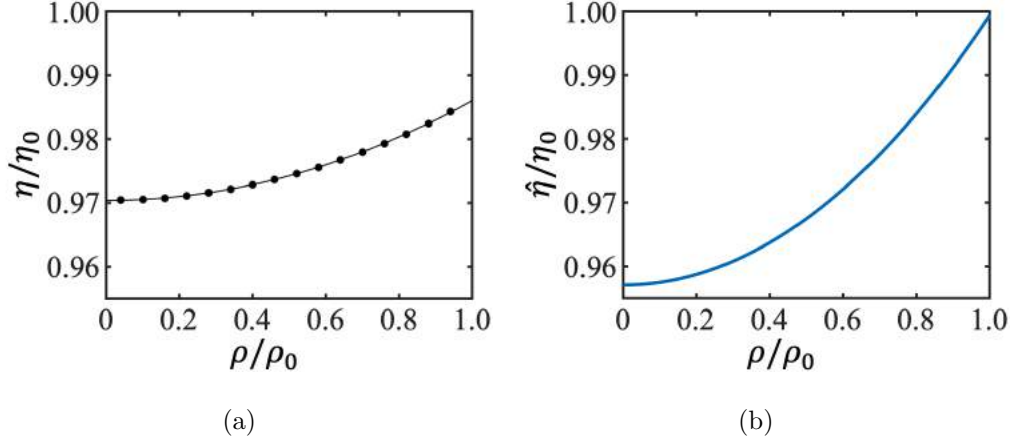

FIG. 3: The distributions of the particle density. (a) The particle density  $\eta$  of the deformed L-J lattice on the sphere at  $\gamma = 1.5\%$ . The numerical data are well fitted by the function in the form of  $\eta(\rho)/\eta(0) = \exp(\alpha K_s \rho^k/2)$ , where  $k = 2.01$  and  $\alpha = 0.35$ .  $K_s$  is the curvature of the spherical substrate. (b) The plot of the density distribution  $\hat{\eta}$  under which the underlying curvature  $K_\ell$  could fully screen the substrate curvature.  $\hat{\eta}(\rho)/\hat{\eta}(0) = \exp(K_s \rho^2/2)$ .  $\rho_0 = 50r_m$ .  $R = 170.1r_m$ .

for the expression of the induced Gaussian curvature:

$$K_\ell = -\frac{1}{2} \Delta \ln \frac{\eta(\rho)}{\eta_0}. \quad (28)$$

The ratio of the densities

$$\frac{\eta(\rho)}{\eta_0} = \left( \frac{dA}{dA_0} \right)^{-1} = [(1 + u_{\rho\rho})(1 + u_{\varphi\varphi})]^{-1}, \quad (29)$$

where  $dA$  and  $dA_0$  are the area elements on the deformed and undeformed disks, respectively.

By inserting Eq. (29) into Eq. (28), we have

$$K_\ell = \frac{1}{2\rho} \frac{d}{d\rho} \left[ \rho \frac{d}{d\rho} \ln \left( (1 + u_{\rho\rho})(1 + u_{\varphi\varphi}) \right) \right]. \quad (30)$$

Up to the linear term of the strain tensor, we obtain Eq.(7) in the main text, which is recorded below:

$$K_\ell = \frac{1}{2} \left[ \frac{1}{\rho} \left( \frac{du_{\rho\rho}}{d\rho} + \frac{du_{\varphi\varphi}}{d\rho} \right) + \left( \frac{d^2 u_{\rho\rho}}{d\rho^2} + \frac{d^2 u_{\varphi\varphi}}{d\rho^2} \right) \right]. \quad (31)$$

### C. Full screening of the substrate curvature $K_s$ by $K_\ell$

It has been shown in the main text that the substrate curvature  $K_s$  is partially screened by the intrinsic curvature underlying the inhomogeneous lattice. A question then arises as

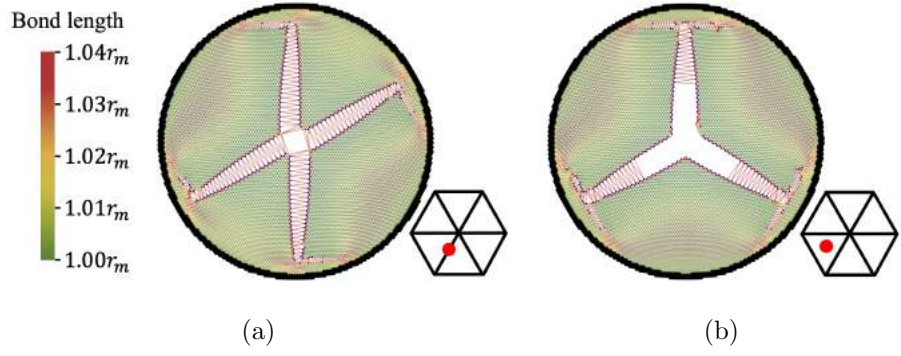

FIG. 4: Fracture patterns with three and four branches by adjusting the relative position of the entire lattice with respect to the center of the crystalline cap. The red dots in the insets indicate the center of the crystalline cap. Both the critical value of  $\gamma$  and the featured turning of the fracture near the boundary are unaffected by the adjustment of the relative position of the lattice.  $\gamma = 7.8\%$ .  $\rho_0 = 50r_m$ .  $R = 81r_m$ .

to the full screening condition. In this subsection, we solve for the density distribution under which  $\hat{K}_\ell = -K_s = -1/R^2$ . By inserting this condition into Eq. (28), we have

$$-\frac{1}{2\rho} \frac{d}{d\rho} \left[ \rho \frac{d}{d\rho} \ln \left( \frac{\eta(\rho)}{\eta_0} \right) \right] = -K_s. \quad (32)$$

The solution is:

$$\frac{\hat{\eta}(\rho)}{\hat{\eta}(0)} = \exp \left( \frac{1}{2} K_s \rho^2 \right), \quad (33)$$

where  $\eta(0)$  is the density at  $\rho = 0$  in the deformed lattice.  $\eta(0)$  shall be distinguished with  $\eta_0$ , which is the constant density in the undeformed lattice. Note that Eq.(33) is valid for  $\eta(0) > 0$ . A typical plot of Eq.(33) is shown in Fig.3(b).

In contrast, the density distribution in the stretched L-J lattice in mechanical equilibrium at  $\gamma = 1.5\%$  conforms to:

$$\frac{\eta(\rho)}{\eta(0)} = \exp \left( \frac{1}{2} \alpha K_s \rho^k \right), \quad (34)$$

where the optimal values for the fitting parameters are:  $k = 2.01$  and  $\alpha = 0.35$ . Equation (34) is plotted in Fig.3(a). By inserting Eq.(34) into Eq.(28), we obtain the induced Gaussian curvature associated with the deformed lattice:

$$K_\ell = -\alpha K_s \rho^{k-2}. \quad (35)$$

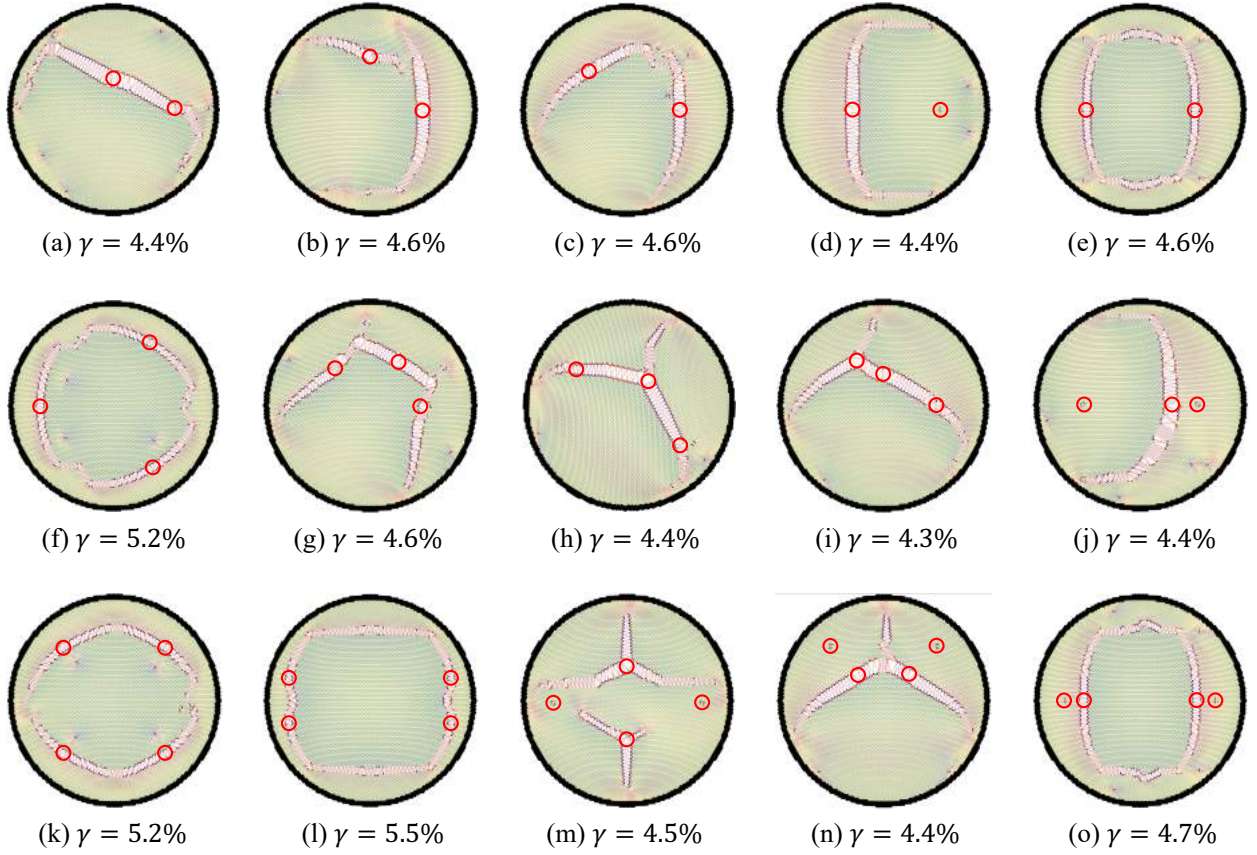

FIG. 5: Fracture patterns by varying the number and locations of the vacancies, as indicated by the empty red circles. The rich patterns demonstrate the active role of microscopic vacancies as stress-controllers in controlling the macroscopic plastic deformation of stressed crystalline membranes.  $\rho_0 = 50r_m$ . The lattice is subject to stronger stretching in the reddish regions.

Due to the smallness of the power  $k-2$  (i.e.,  $k-2 = 0.01$ ), the value of  $K_\ell$  is almost constant over the disk. We thus obtain the excess curvature as:

$$\frac{K_\ell + K_s}{K_s} \approx 0.65, \quad (36)$$

which is consistent with the theoretical result in Eq.(8) in the main text.

#### IV. FRACTURE OF THE HIGHLY STRETCHED CRYSTALLINE CAP

In this section, we present more information about the fracture of highly stretched crystalline caps in the presence of vacancies.

In Fig.3(a) in the main text, we have presented a typical fracture pattern in the presence

of a single vacancy at the center of the crystalline cap. By adjusting the relative position of the entire lattice with respect to the center of the cap, we observe fracture patterns with three and four branches, as shown in Fig. 4. The red dots in the insets of Fig. 4 indicate the center of the crystalline cap. While the specific number of branches in the fracture is sensitive to the relative position of the lattice, both the critical value of  $\gamma$  and the featured turning of the fracture near the boundary are unaffected, indicating the limited influence of the crystalline structure on the rupture mode.

In Fig. 5, we present more examples of fracture patterns by varying the number and locations of the vacancies. The locations of the vacancies are indicated by the empty red circles in Fig. 5. The rich fracture patterns exhibit the active role of microscopic vacancies in controlling the macroscopic plastic deformation of stressed crystalline membranes, and suggest the promising potential of vacancies as stress-controllers.

- 
- [1] J. A. Snyman and D. N. Wilke, *Practical Mathematical Optimization* (Springer, New York, 2005).
  - [2] Z. Yao and M. Olvera de la Cruz, Phys. Rev. Lett. **116**, 148101 (2016).
  - [3] L. D. Landau and E. Lifshitz, *Theory of Elasticity* (Pergamon, London, 1959).
  - [4] G. N. Greaves, A. L. Greer, R. S. Lakes, and T. Rouxel, Nat. Mater. **10**, 823 (2011).
  - [5] T. Belytschko, W. K. Liu, B. Moran, and K. Elkhodary, *Nonlinear Finite Elements for Continua and Structures* (John Wiley & Sons, New York, 2013).
  - [6] D. J. Struik, *Lectures on Classical Differential Geometry* (Dover Publications, New York, 1988), 2nd ed.
